# Supplementary material for: Universal mechanical instabilities in the energy landscape of amorphous solids: evidence from athermal quasistatic expansion
Source: arXiv:2109.06902 ancillary file (2021-09-14)
Supplement: Supplementary file 1 [file supplementary.pdf]

# Supplementary Information: Universal mechanical instabilities in the energy landscape of amorphous solids: evidence from athermal quasistatic expansion

Umang A. Dattani,[1,2] Smarajit Karmakar,[3] and Pinaki Chaudhuri[1,2]

[1] *The Institute of Mathematical Sciences, CIT Campus, Taramani, Chennai 600113, India*
[2] *Homi Bhabha National Institute, Anushaktinagar, Mumbai 400094, India*
[3] *Tata Institute of Fundamental Research, 36/P, Gopanpally Village, Serilingampally Mandal,Ranga Reddy District, Hyderabad, 500107, Telangana, India*

## DETAILS OF MODEL AND METHODS

### Model

For our study, we use the 2DMKA binary Lennard-Jones glass-forming mixture, which has 65 : 35 composition of the two species, labelled $A$ and $B$, with interaction parameters – $\sigma_{AA} = 1.0$, $\sigma_{BB} = 0.88$, $\sigma_{AB} = 0.8$, $\epsilon_{AA} = 1.0$, $\epsilon_{BB} = 0.5$, $\epsilon_{AB} = 1.5$ [1]. The interaction potential, smoothened up to first two derivatives, for particles $i$ and $j$ is the following:

$$V(r) = 4\epsilon_{ij}\left[\left(\frac{\sigma_{ij}}{r_{ij}}\right)^{12} - \left(\frac{\sigma_{ij}}{r_{ij}}\right)^{6}\right] + C_0 + C_2\left(\frac{r_{ij}}{\sigma_{ij}}\right)^{2} + C_4\left(\frac{r_{ij}}{\sigma_{ij}}\right)^{4} \tag{1}$$

, where $i$ and $j$ would correspond to either of the labels $A$ or $B$. The constants $C_0$, $C_2$ and $C_4$ are determined by requiring the potential and its first two derivates to be zero at the cutoff $r = 2.5\sigma_{ij}$. The simulations have been performed for a variety of system sizes ranging from $N = 10^3$ to $N = 10^5$.

### Initial State

To prepare initial states for our study, we first equilibriate the system at $T = 1.0$ (in LJ units), which is in the liquid regime, followed by cooling at a constant rate of $10^{-4}$ per MD timestep to a final temperature of $T = 0.01$, which is in the glassy regime. The corresponding glass transition (Kauzmann) temperature of the model system is at 0.30 **(Find reference.)**. The athermal states used in our study are generated by obtaining inherent structure states corresponding to the glassy configurations at $T = 0.01$, via conjugate gradient (CG) minimization.

### Athermal Quasistatic Expansion

To explore cavitation in the limit of temperature $T \to 0$ and strain rate $\dot{\gamma} \to 0$, we use the Athermal Quasistatic Expansion(AQE) method [2]. In each step, a constant isotropic volume strain is applied on the system by rescaling the lengths of the box by a factor $1 + \epsilon$, followed by remapping of coordinates. The energy of the strained configuration is then minimized using the CG algorithm[3]. The minimization stops when the energy of the system in two successive iterations, $\mid \Delta E \mid / \mid E \mid < 10^{-16}$. The values of $\epsilon$ are varied from $10^{-4}$ to $10^{-9}$. This protocol helps us effectively explore the potential energy landscape, during cavitation, similar to AQS protocol [4]. All these simulations are done using LAMMPS [5].

### Eigenvalue and Eigenvectors of Hessian

For a system of $N$ particles interacting via a pairwise potential $\phi(r)$, the potential energy is given by,

$$U(\boldsymbol{r}_1, \boldsymbol{r}_2, \dots \boldsymbol{r}_N) = \sum_{i=1}^{N} \sum_{j=1; i\neq j}^{N} \phi(\mid \boldsymbol{r}_i - \boldsymbol{r}_j \mid)$$

The Hessian matrix of the potential energy for a pairwise potential can be reduced to[6],

$$\mathcal{H}^{ij}_{\alpha\beta} = \frac{\partial^2 U}{\partial \boldsymbol{r}^i_\alpha \, \partial \boldsymbol{r}^j_\beta} = -\left( \frac{\phi^{ij}_{rr}}{(r^{ij})^2} - \frac{\phi^{ij}_r}{(r^{ij})^3} \right) r^{ij}_\alpha r^{ij}_\beta - \delta_{\alpha\beta} \frac{\phi^{ij}_r}{r^{ij}} \tag{2}$$

Where, $r^{ij}_0 = x^i - x^j$, $r^{ij}_1 = y^i - y^j$, $\phi_r = \partial\phi/\partial r$ and $\phi_r = \partial^2\phi/\partial r^2$

The eigevalues and eigenfunctions of the Hessian are computed using LAPACKE[7].

### Statistics

The statistics of jumps i.e. $P(\Delta P)$ and $P(\Delta U)$ are recorded with a step size $\epsilon = 5 \times 10^{-3}$ upto a density of $\rho_0 = 0.9825$ (200 expansion steps). The number of independent realizations for each of the system sizes is given in the table below.

| $N$ | Number of independent realizations |
|---|---|
| 1000 | 4996 |
| 5000 | 1844 |
| 25000 | 1207 |
| 100000 | 491 |

# SUPPLEMENTARY PLOTS

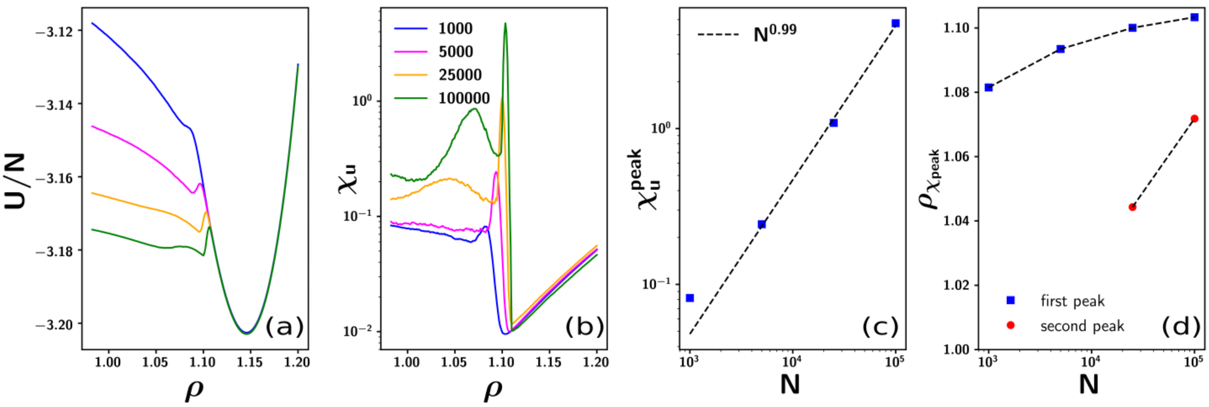


FIG. 1: (a) Potential energy per particle variation with density averaged over the ensemble. (b) The corresponding susceptibility of energy for different system sizes $\chi_u = (1/N)\left[\langle U^2\rangle - \langle U\rangle^2\right]$. (c) The susceptibility values at the peak for different system sizes. Similar to $\chi_p^{peak}$ [see main text], $\chi_u^{peak} \sim N$. (d) Density values at which the two peaks in susceptibility occur, for different system sizes.

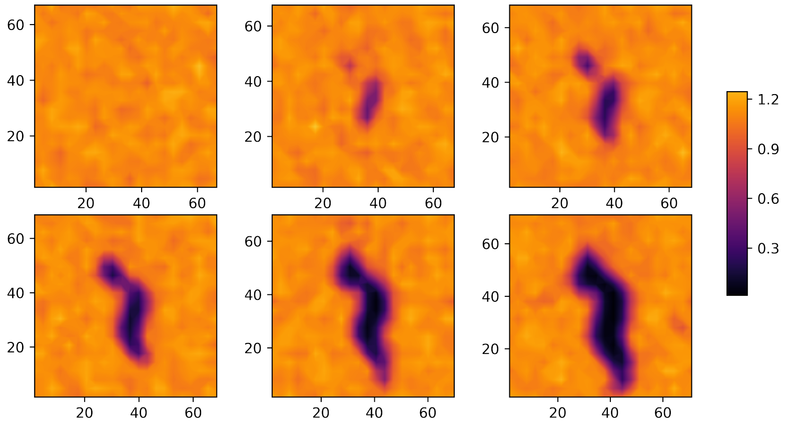

FIG. 2: $N = 5000$. Coarse-grained density field at the points marked in red in Fig.2a and 2b of main text, with density increasing from left to right, and from top to bottom. The coarse-grained fields are constructed following the procedure described in Ref.[8]

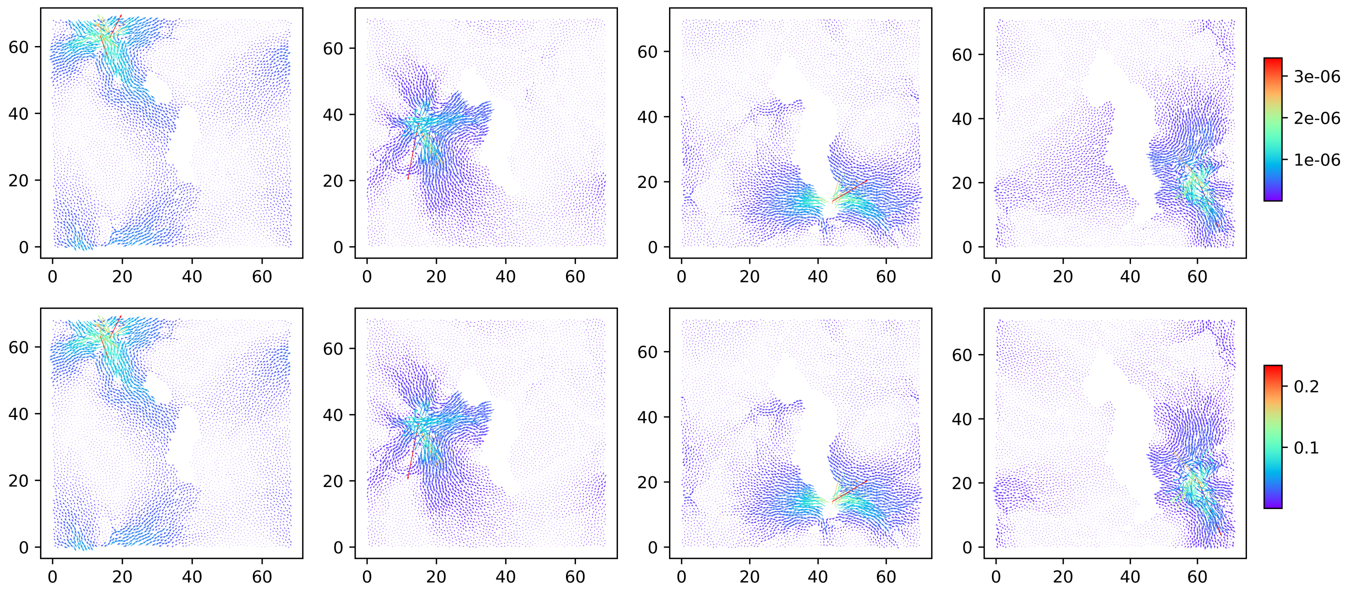

FIG. 3: $N = 5000$. (Top) For the density locations marked in Fig.2(a) of the main text, after the main cavitation event, maps of non-affine displacements across the pressure jump occurring there. (Bottom) Maps of eigenfunctions of the Hessian matrix at the same points. In both cases, density decreases from left to right.

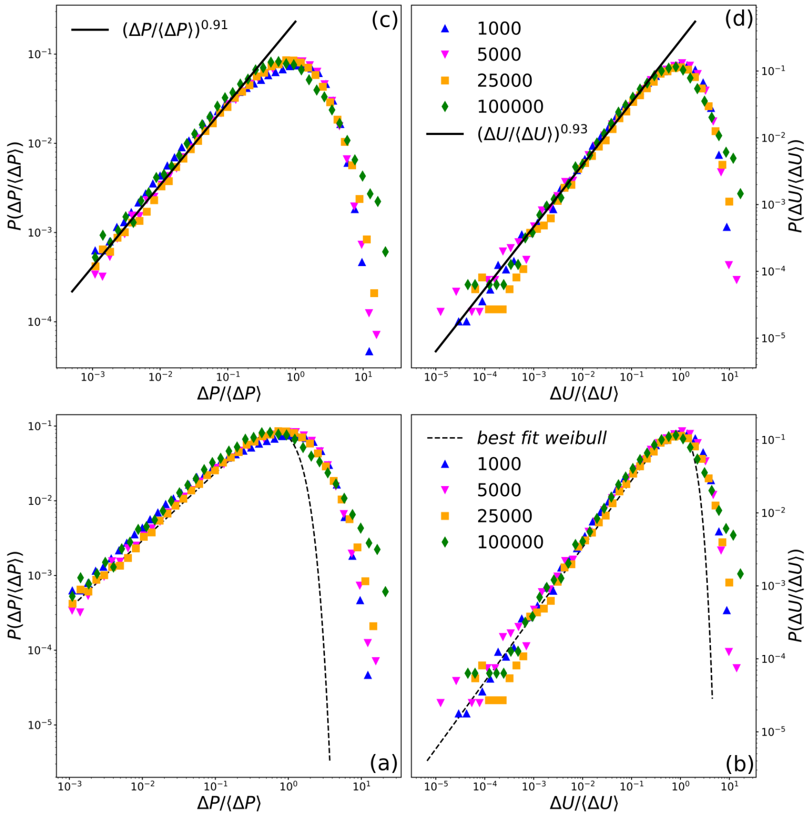


FIG. 4: (The collapse of post-yield distributions on scaling with mean size of (a) pressure jumps and (b) energy jumps. Also shown are power-law fits to the collapsed data in the regime where the variable has small value. (c)-(d) Best fit with Weibull distributions to the collapsed data shown in (a) & (b), where the variable has small value. Fit parameters: (c) $k = 1.91$ and $\lambda = 1.0907$ (d) $k = 1.93$ and $\lambda = 1.3293$, for the Weibull function $f(x) = \frac{k}{\lambda}\left(\frac{x}{\lambda}\right)^{k-1} e^{-(x/\lambda)^k}$

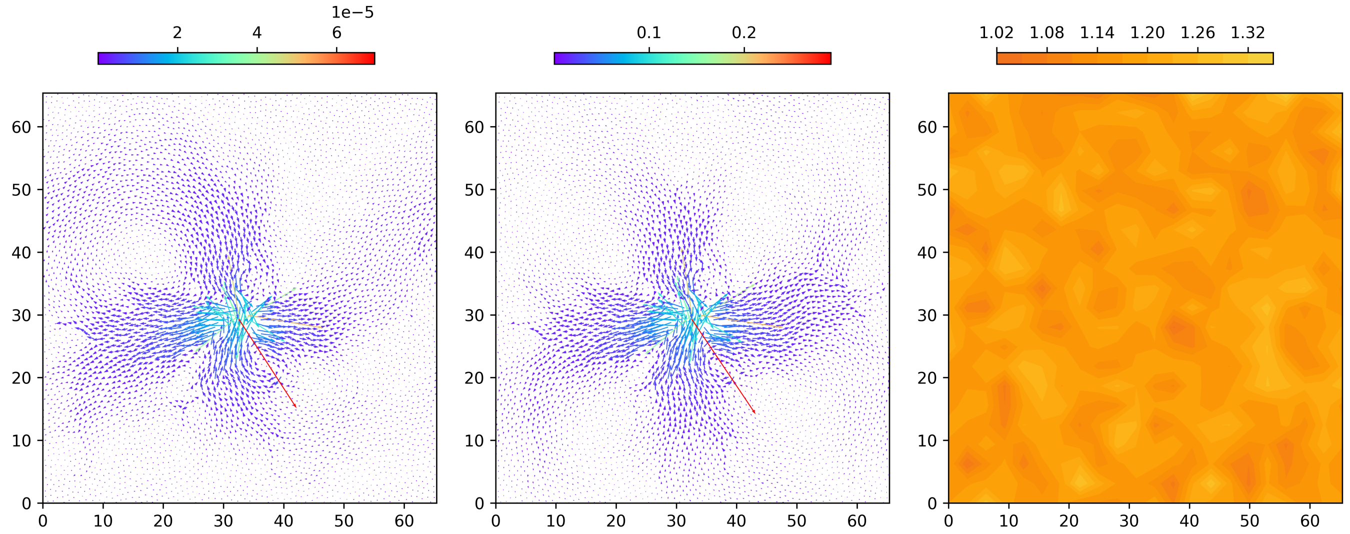


FIG. 5: $N = 5000$. First irreversible event during AQE. (a) Map of non-affine displacemnts for the first jump shown in Fig.4 of the main text. b) Eigenvector of the lowest non-zero eigenvalue at the same density ($\rho = 1.168$), prior to jump. (c) Coarse-grained density field after the first jump, displaying spatial homogeneity.

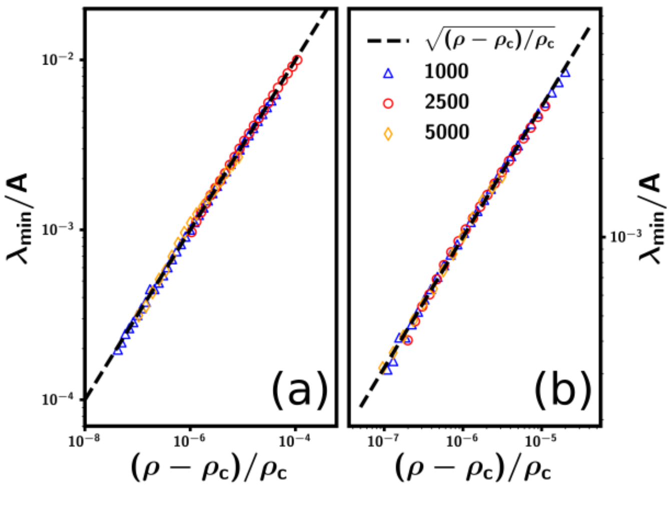


FIG. 6: For different system sizes, evidence of square root singularity for the lowest eigenvalue of the Hessian, $\lambda_{min}$ in the (a) pre-yield and (b) post-yield regimes. The $\lambda_{min}$s have been scaled appropriately so that they all fall on the same line.

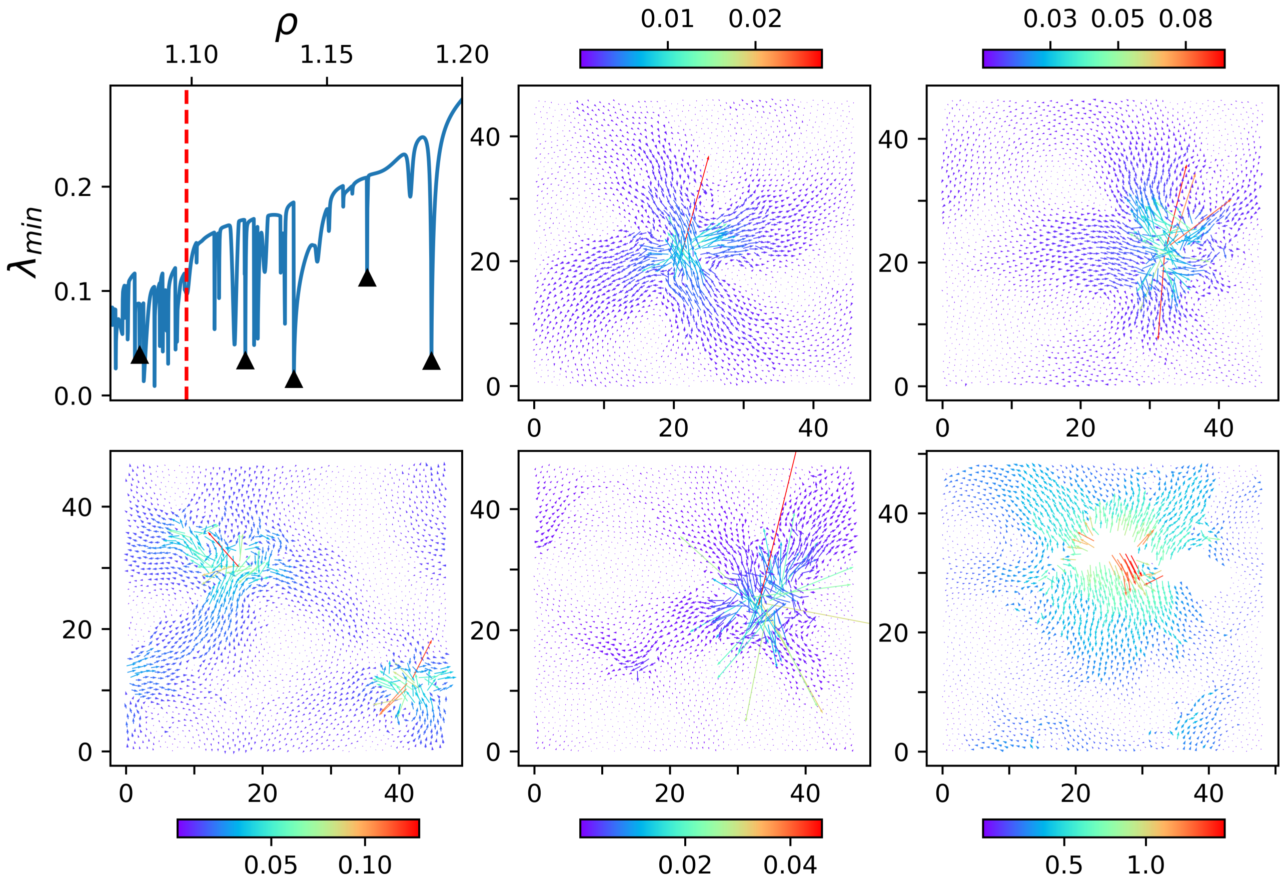


FIG. 7: $N = 2500$. (a): $\lambda_{min}$ vs $\rho$ during athermal quasistatic exapansion; the red line marks the point at which density inhomogeneity first appears during the expansion. (b)-(f): Maps of non-affine displacements corresponding to the plastic events marked in black in (a), in order of decreasing density with expansion. Once the density inhomogeneity appears in the system, the quadrupolar structure of non-affine displacements gets transformed; see (f).

[1] W. Kob and H. C. Andersen, Physical Review E **51**, 4626 (1995).
[2] Y. E. Altabet, F. H. Stillinger, and P. G. Debenedetti, The Journal of Chemical Physics **145**, 211905 (2016).
[3] E. Polak and G. Ribiere, ESAIM: Mathematical Modelling and Numerical Analysis - Modélisation Mathématique et Analyse Numérique **3**, 35 (1969), URL `http://www.numdam.org/item/M2AN_1969__3_1_35_0/`.
[4] C. E. Maloney and A. Lemaître, Phys. Rev. E **74**, 016118 (2006), URL `https://link.aps.org/doi/10.1103/PhysRevE.74.016118`.
[5] S. Plimpton, Journal of Computational Physics **117**, 1 (1995), ISSN 0021-9991, URL `https://www.sciencedirect.com/science/article/pii/S002199918571039X`.
[6] S. Karmakar, E. Lerner, and I. Procaccia, Phys. Rev. E **82**, 026105 (2010), URL `https://link.aps.org/doi/10.1103/PhysRevE.82.026105`.
[7] E. Anderson, Z. Bai, C. Bischof, S. Blackford, J. Demmel, J. Dongarra, J. Du Croz, A. Greenbaum, S. Hammarling, A. McKenney, et al., *LAPACK Users' Guide* (Society for Industrial and Applied Mathematics, Philadelphia, PA, 1999), 3rd ed., ISBN 0-89871-447-8 (paperback).
[8] V. Testard, L. Berthier, and W. Kob, Physical review letters **106**, 125702 (2011).
